# Supplementary material for: Toward a Better Understanding of Fourier Neural Operators from a Spectral Perspective
Source: arXiv:2404.07200 source file (2024-10-09)
Supplement: Supplementary file 1 [file ablation_resolution.tex]

\section{SpecB-FNO Resolution Property}
\label{sec:appendix_resolution}

{\color{red} TBD}

\begin{wrapfigure}{o}{0.3\textwidth}
  \centering
  \includegraphics[width=0.3\textwidth]{example-image}
  \vspace{-5pt}
  \caption{SpecB-FNO Resolution Property.}
  \vspace{-5pt}
  \label{fig:resolution}
\end{wrapfigure}

Figure \ref{fig:resolution} examines the resolution-invariant property of both FNO and SpecB-FNO, as FNO is designed to be resolution-invariant.
FNO is specifically crafted to be tested on higher-resolution data than that used for training. Moreover, FNO can also be evaluated on lower-resolution data as long as the frequency modes of the model do not exceed the maximum frequency modes of the test data. 
%Maintaining consistent model hyperparameters across diverse resolutions ensures that the model trained with S=421 can still be tested when S=85. 
Figure \ref{fig:resolution} illustrates that optimal performance is achieved when training FNO on data with the same resolution as the testing data. Training on resolutions higher or lower than the testing data negatively impacts testing performance. 
% The enhancements facilitated by SpecB-FNO can extend to close resolutions, with the magnitude of improvements diminishing as the resolution gap widens.
SpecB-FNO's improvements extend across various testing resolutions, with more significant enhancements observed at closer resolutions.

\section{Detailed Darcy Flow Evaluations}
\label{sec:appendix_darcy}

{\color{red} TBD}

We demonstrate the detailed results for Figure \ref{fig:resolution} in Table \ref{tab:darcy_full} and further include the improvement from FNO to SpecB-FNO. The experimental result indicates that the enhancements facilitated by SpecB-FNO can extend to close resolutions, with the magnitude of improvements diminishing as the resolution gap widens.

\begin{table*}[!htbp]
\caption{Complete relative error ($1\times 10^{-3}$) comparison on Darcy flow between FNO and SpecB-FNO with FNO-skip. Imp. indicates the relative improvement from FNO to SpecB-FNO.}
\resizebox{\textwidth}{!}{
\begin{tabular}{l | *{3}{c} | *{3}{c} | *{3}{c} | *{3}{c}}  
\toprule[+1pt]
\multirow{2}{*}{Train} & \multicolumn{3}{c|}{Test: $S$=85} & \multicolumn{3}{c|}{Test $S$=141} & \multicolumn{3}{c|}{Test: $S$=211} & \multicolumn{3}{c}{Test: $S$=421} \\
\cmidrule(lr){2-4} \cmidrule(lr){5-7} \cmidrule(lr){8-10} \cmidrule{11-13}
& FNO & SpecB-FNO &  Imp. (\%) & FNO & SpecB-FNO &  Imp. (\%) & FNO & SpecB-FNO &  Imp. (\%) & FNO & SpecB-FNO &  Imp. (\%) \\
\midrule 
$S$=85  & \bf{9.46} $\pm$ 0.08 & \bf{4.89} $\pm$ 0.04 & \bf{48.3} & 13.75     $\pm$ 0.22 & 11.17     $\pm$ 0.17 & 18.8 & 17.62     $\pm$ 0.30 & 15.70     $\pm$ 0.27 & 10.9 & 21.87     $\pm$ 0.43 & 20.33     $\pm$ 0.33 & 7.0 \\
$S$=141 & 13.97     $\pm$ 0.35 & 11.21     $\pm$ 0.22 & 19.8 & \bf{9.16} $\pm$ 0.10 & \bf{4.00} $\pm$ 0.08 & \bf{56.3} & 10.42     $\pm$ 0.16 & 6.36      $\pm$ 0.05 & 39.0 & 13.50     $\pm$ 0.16 & 10.58     $\pm$ 0.16 & 21.6 \\
$S$=211 & 17.99     $\pm$ 0.47 & 15.84     $\pm$ 0.24 & 12.0 & 10.51     $\pm$ 0.13 & 6.27      $\pm$ 0.05 & 40.3 & \bf{9.19} $\pm$ 0.06 & \bf{3.70} $\pm$ 0.04 & \bf{59.7} & 10.48     $\pm$ 0.10 & 6.19      $\pm$ 0.05 & 40.9 \\
$S$=421 & 22.46     $\pm$ 0.60 & 20.69     $\pm$ 0.29 & 7.9  & 13.73     $\pm$ 0.29 & 10.70     $\pm$ 0.18 & 22.1 & 10.61.    $\pm$ 0.07 & 6.32      $\pm$ 0.13 & 40.4 & \bf{9.32} $\pm$ 0.10 & \bf{3.65} $\pm$ 0.02 & \bf{60.8} \\
\bottomrule[+1pt]
\end{tabular}}
\label{tab:darcy_full}
\end{table*}
